# Supplementary material for: Artificial diffusion for convective and acoustic low Mach number flows II: Application to Liou-Steffen, Zha-Bilgen and Toro-Vasquez convection-pressure flux splittings
Source: arXiv:2303.10740 source file (2023-03-19)
Supplement: Supplementary file 1 [file ausm2fds_proof.tex]

General form of AUSM scheme
\begin{equation}
\hat{f}=\left\{ f\right\}- \dot{c}/2 \llbracket \varphi \rrbracket - c_d \llbracket -p_d n
\end{equation}
\begin{equation}
\dot{c}=\dot{u}
\end{equation}
\begin{equation}
    \hat{f}=\left\{ f\right\}- \left|A\right|\llbracket q\rrbracket=
    \dot{u}I\llbracket \varphi\rrbracket
    +\varphi 
    \left( \begin{matrix} \nu _p^u & \nu_u^u \end{matrix}\right)\left(
   \llbracket p\rrbracket \\
   \llbracket u \rrbracket 
    \right)
    +\left( \begin{matrix} 0\\1\\0\\0\end{matrix}\right)
    \left( \begin{matrix} \nu _p^p& \nu_u^p \end{matrix}\right)\left(
   \llbracket p\rrbracket \\
   \llbracket u \rrbracket 
    \right)
\end{equation}
where
\begin{equation}
    \varphi =\rho \left(\begin{matrix}
    1 \\ u \\ v \\ h
    \end{matrix}
    \right)
\end{equation}
Define
\begin{equation}
    \llbracket p\rrbracket= \rho a \llbracket \phi \rrbracket
\end{equation}
\begin{equation}
    \hat{f}=\left\{f\right\}-
    \left(
   \begin{matrix} 
   \dfrac{u}{2} \llbracket \rho \rrbracket+
   \nu_u^u\rho \llbracket u \rrbracket+
   \nu_p^u\rho \llbracket p \rrbracket \\
   \dfrac{u}{2} \llbracket \rho u \rrbracket+
   \nu_u^u\rho u \llbracket u \rrbracket+
   \nu_p^u\rho u \llbracket p \rrbracket +
   \nu_p^p\llbracket p\rrbracket+
   \nu_u^p\llbracket u\rrbracket \\
   \dfrac{u}{2} \llbracket \rho v\rrbracket+
   \nu_u^u\rho v \llbracket u \rrbracket+
   \nu_p^u\rho v \llbracket p \rrbracket \\
   \dfrac{u}{2} \llbracket \rho h\rrbracket+
   \nu_u^u\rho h \llbracket u \rrbracket+
   \nu_p^u\rho h \llbracket p \rrbracket
   \end{matrix} 
    \right)
\end{equation}

\begin{equation}
    \hat{f}=\left\{f\right\}-
    \left(
    \begin{matrix}
    \dfrac{u}{2} & 0 & 0 & 0 \\
    0 & \dfrac{u}{2} & 0 & 0 \\
    0 & 0 & \dfrac{u}{2} & 0 \\
    0 & 0 & 0 & \dfrac{u}{2} \\
    \end{matrix}
    \right)
    \left(
   \begin{matrix}
   \llbracket \rho \rrbracket \\
   \llbracket \rho u \rrbracket \\
   \llbracket \rho v \rrbracket \\
   \llbracket \rho h\rrbracket \\
   \end{matrix} 
    \right)
-
    \left(\begin{matrix}
     \nu_p^u \rho & \nu_u^u \rho \\
     \nu_p^u \rho u &\nu_p^p & \nu_u^u \rho u +\nu_u^p \\
     \nu_p^u \rho v & \nu_u^u \rho v  \\
     \nu_p^u \rho h & \nu_u^u \rho h \\
    \end{matrix}\right)
   \begin{matrix}
   \llbracket p \rrbracket
   \llbracket u \rrbracket
   \end{matrix} 
\end{equation}
Transformation jacobians
\begin{equation}
\dfrac{\partial q^s}{\partial q^c}=
\dfrac{1}{\rho a}\left( \begin{matrix}
\Gamma k & -\Gamma u & -\Gamma v & \Gamma \\
-u a &  a & 0 & 0 \\
-v a &  0 & a & 0 \\
\Gamma k -a^2 & -\Gamma u & -\Gamma v & \Gamma
\end{matrix}\right)
\end{equation}
\begin{equation}
\dfrac{\partial \varphi}{\partial q^s}=
\dfrac{\rho}{a}\left( \begin{matrix}
1 &  0 & 0 & -1 \\
 u &  a & 0 & -u \\
v  &  0 & a & -v \\
\dfrac{\gamma a^2}{\Gamma}+k & u a & v a& -k
\end{matrix}
\right)
\end{equation}
Note
\begin{equation}
\dfrac{\partial q^s}{\partial q^c}
\dfrac{\partial \varphi}{\partial q^s}=
\left(
\begin{matrix}
\gamma & 0 & 0 & 0 \\
     0 & 1 & 0 & 0 \\
     0 & 0 & 1 & 0 \\
     \gamma-1 & 0 & 1 & 0
\end{matrix}
\right)
\end{equation}
\begin{equation}
   A\llbracket q\rrbracket  \left[
   \dot{u} 
   \left(
   \begin{matrix}
    \gamma & 0 & 0 & 1\\
    0 & 1 & 0 & 0 \\
    0 & 0 & 1 & 0 \\
    \gamma-1 &  0 & 0 & 1
    \end{matrix}
    \right)
    +
    \left(
   \begin{matrix}
    \rho a^2 \nu_p^u & a \nu_u^u & 0 & 0\\
    0 & 0 & 0 & 0 \\
    0 & 0 & 0 & 0 \\
    0 & 0 & 0 & 0
    \end{matrix}
    \right)
    +
    \left(
   \begin{matrix}
    -\Gamma \frac{u}{a}\\
    1 \\
    0 \\
    -\Gamma \dfrac{u}{a}
    \end{matrix}
    \right)\left(\begin{matrix} 0 & a \nu_p^p & \dfrac{\nu_u^p}{\rho} & 0\end{matrix}\right)
    \right]
    \left(
    \begin{matrix}
    \llbracket \phi \rrbracket \\
    \llbracket u \rrbracket \\
    \llbracket v \rrbracket \\
    \llbracket \zeta \rrbracket \\
    \end{matrix} 
    \right)
\end{equation}
\subsection{$\phi$ equation}
\begin{equation}
\left(\dot{u}\gamma\left(1-\nu_p^p\right)+ \rho a^2 \nu_p^u \right)\llbracket \phi \rrbracket
+\left( a\nu_u^u -\Gamma \nu_u^p \dfrac{u}{a}\right)\llbracket u\rrbracket
\end{equation}
\subsection{$u$ equation}
\begin{equation}
\left(a \nu_p^p\right)\llbracket \phi \rrbracket
+\left( \dot{u} + \dfrac{\nu_u^p}{\rho}\right)\llbracket u\rrbracket
\end{equation}
\subsection{$v$ equation}
\begin{equation}
\dot{u}\llbracket v\rrbracket
\end{equation}
\subsection{$\zeta$ equation}
\begin{equation}
\left(\dot{u}\left(\gamma-1\right)- \Gamma u \nu_p^p \right)\llbracket \phi \rrbracket 
- \dfrac{\gamma u \nu _u^p}{\rho a}\llbracket u \rrbracket + u\llbracket \zeta \rrbracket
\end{equation}
\begin{equation}
\dot{u}\left(\gamma-1\right)\left(1- \nu_p^p \right)\llbracket \phi \rrbracket 
- \dfrac{\gamma u \nu _u^p}{\rho a}\llbracket u \rrbracket + u\llbracket \zeta \rrbracket
\end{equation}

\subsection{Introduce symmetrising variables}
Proceed column by column
\begin{equation}
   \left( \dfrac{\partial q^s}{\partial q^c}\right) \varphi \left(\begin{matrix}\nu_p^u && \nu_u^u \end{matrix}\right)\left(\begin{matrix}
   \llbracket p\rrbracket \\
   \llbracket u \rrbracket \end{matrix}\right)=
   \left( \dfrac{\partial q^s}{\partial q^c}\right) \varphi \left(\begin{matrix}\rho a \nu_p^u && \nu_u^u \end{matrix}\right)\left(\begin{matrix}
   \llbracket \phi \rrbracket \\
   \llbracket u \rrbracket \end{matrix}\right)
\end{equation}
\begin{equation}
   \left( \dfrac{\partial q^s}{\partial q^c}\right) \varphi =
   \dfrac{\rho}{\rho a}\left( 
  \begin{matrix}
  \Gamma k & -\Gamma u & -\Gamma v & \Gamma \\
  -u a & a & 0 & 0\\
  -v a & 0 & a & 0 \\
  \Gamma h -k & -\Gamma a & -\Gamma v & \Gamma
  \end{matrix} 
   \right)
   \left(
   \begin{matrix}
   1 \\ u \\ v \\ h
   \end{matrix}
   \right)=
   \dfrac{\Gamma}{a}\left( \begin{matrix}
   h-k \\ 0 \\ 0 \\ h-k-\dfrac{a^2}{\Gamma} 
   \end{matrix}\right)
\end{equation}
Note
\begin{equation}
    h-k= \dfrac{a^2}{\Gamma}
\end{equation}
hence
\begin{equation}
   \left( \dfrac{\partial q^s}{\partial q^c}\right) \varphi =
   \left( \begin{matrix}
   a \\ 0 \\ 0 \\ 0
   \end{matrix}\right)
\end{equation}
\begin{equation}
   \left( \dfrac{\partial q^s}{\partial q^c}\right) \varphi \left(\begin{matrix}\nu_p^u && \nu_u^u \end{matrix}\right)\left(\begin{matrix}
   \llbracket p\rrbracket \\
   \llbracket u \rrbracket \end{matrix}\right)=
   \left( \begin{matrix}
   1 \\ 0 \\ 0 \\ 0
   \end{matrix}\right)
   \left( \dfrac{\partial q^s}{\partial q^c}\right) \varphi \left(\begin{matrix}\rho a \rho a^2 \nu_p^u && a \nu_u^u \end{matrix}\right)\left(\begin{matrix}
   \llbracket \phi \rrbracket \\
   \llbracket u \rrbracket \end{matrix}\right)
\end{equation}

\begin{equation}
   \left( \dfrac{\partial q^s}{\partial q^c}\right) 
  \left(\begin{matrix}0\\1\\0\\0\end{matrix}\right) 
   \left(\begin{matrix}\nu_p^u && \nu_u^u \end{matrix}\right)\left(\begin{matrix}
   \llbracket p\rrbracket \\
   \llbracket u \rrbracket \end{matrix}\right)=
   \left( \dfrac{\partial q^s}{\partial q^c}\right) 
  \left(\begin{matrix}0\\1\\0\\0\end{matrix}\right) 
   \left(\begin{matrix}\rho a \nu_p^u && \nu_u^u \end{matrix}\right)\left(\begin{matrix}
   \llbracket \phi \rrbracket \\
   \llbracket u \rrbracket \end{matrix}\right)
\end{equation}
\begin{equation}
   \left( \dfrac{\partial q^s}{\partial q^c}\right) \left(\begin{matrix}
   0 \\ 1 \\ 0 \\ 0 \end{matrix}\right) =
   \dfrac{\rho}{\rho a}\left( 
  \begin{matrix}
  \Gamma k & -\Gamma u & -\Gamma v & \Gamma \\
  -u a & a & 0 & 0\\
  -v a & 0 & a & 0 \\
  \Gamma h -k & -\Gamma a & -\Gamma v & \Gamma
  \end{matrix} 
   \right)
   \left(
   \begin{matrix}
   0 \\ 1 \\ 0 \\ 0
   \end{matrix}
   \right)=
   \dfrac{1}{\rho a}\left( \begin{matrix}
   -\Gamma u \\ a \\ 0 \\ -\Gamma u 
   \end{matrix}\right)
\end{equation}
\begin{equation}
   \left( \dfrac{\partial q^s}{\partial q^c}\right) \left(\begin{matrix}
  0 \\ 1 \\ 0 \\ 0  \end{matrix}\right)\left(\begin{matrix}
   \llbracket p\rrbracket \\
   \llbracket u \rrbracket \end{matrix}\right)=
   \dfrac{1}{\rho a}\left( \begin{matrix}
   -\Gamma u \\ a \\ 0 \\ -\Gamma u
   \end{matrix}\right)
   \left( \dfrac{\partial q^s}{\partial q^c}\right) \varphi \left(\begin{matrix}\rho a^2 \nu_p^u && a \nu_u^u \end{matrix}\right)\left(\begin{matrix}
   \llbracket \phi \rrbracket \\
   \llbracket u \rrbracket \end{matrix}\right)
\end{equation}
