# Supplementary material for: Artificial diffusion for convective and acoustic low Mach number flows II: Application to Liou-Steffen, Zha-Bilgen and Toro-Vasquez convection-pressure flux splittings
Source: arXiv:2303.10740 source file (2023-03-19)
Supplement: Supplementary file 2 [file ausm_scheme_comparison.tex]

\subsection{AUSM$^+$-up}
The interface velocity in AUSM+up is:
\begin{equation}
    u_{1/2} =  a\mathcal{M}^{+}_{(4)}(M_L)
             + a\mathcal{M}^{-}_{(4)}(M_R)
             - \frac{1-M^2}{4 f_a} \frac{\llbracket p \rrbracket}{\rho a}
\end{equation}
Where $f_a=M_0(2-M_0)$, and $M_0$ is the local Mach number clamped between $1$ and a cut-off value $M_{co}$.
Any arithmetic coefficients have been taken as the values given in the original paper.
The fourth order Mach splittings $\mathcal{M}^{\pm}_{(4)}$ are given, for subsonic flow, by:
\begin{equation}
    \mathcal{M}^{\pm}_{(4)}(M) = \pm \frac{1}{8}(3 \pm 4M + M^4)
\end{equation}
Substituting (\ref{eq:mach_splitting_4th}) into (\ref{eq:ausmpup:interface_velocity}) and discarding higher order terms in $M$, the low Mach number approximation to the interface velocity is:
\begin{equation}
    u_{1/2} = \{u\} - \frac{\llbracket p \rrbracket}{8\rho a M} + \mathcal{O}(M^3)
\end{equation}
From which it can be see that:
\begin{equation}
    \nu_u \approx 0,
    \quad
    \nu_p = \frac{1}{4\rho a M} \sim \mathcal{O}(M^0)
\end{equation}
The interface pressure is given by:
\begin{equation}
    p_{1/2} =  \mathcal{P}^{+}_{(5)}(M_L)p_L
             + \mathcal{P}^{-}_{(5)}(M_R)p_R
             - \frac{3}{4}\mathcal{P}^{+}_{(5)}(M_L)\mathcal{P}^{-}_{(5)}(M_R)\rho f_a a \llbracket u \rrbracket
\end{equation}
The calculation of the fifth order pressure splittings $\mathcal{P}^{\pm}_{(5)}$ relies on a parameter $\alpha$ which, at low Mach number is approximately $-\frac{3}{4}$.
Using this approximation, the pressure splittings are:
\begin{equation}
    \mathcal{P}^{\pm}_{(5)}(M) = \frac{1}{4} ( 2 \pm 5M^3 \mp 3M^5 )
\end{equation}
Substituting (\ref{eq:pressure_splitting_5th_convective}) into (\ref{eq:ausmpup:interface_pressure}) and discarding higher order terms in $M$, the low Mach number approximation to the interface pressure is:
\begin{equation}
    p_{1/2} \approx \{p\} - \bigg( \frac{3\rho a M}{8} + \frac{15\rho a M^2}{4} \bigg)\llbracket u \rrbracket + \mathcal{O}(M^4)
\end{equation}
The second term in the brackets is an order of $M$ smaller than the first, so we neglect it in the limit to find:
\begin{equation}
    \mu_p \approx 0,
    \quad
    \mu_p \approx -\frac{3\rho a M}{8} \sim \mathcal{O}(M^0)
\end{equation}
Collecting (\ref{eq:ausmpup_nu_convective}) and (\ref{eq:ausmpup_mu_convective}) together, the diffusion matrix of AUSM$^+$-up scales as:
\begin{equation}
    \underline{\underline{A}} \sim \mathcal{O}
    \begin{matrix}
    \begin{pmatrix}
        M^{-2} & 0     \\
        0      & M^{0} \\
    \end{pmatrix}
    \end{matrix}
\end{equation}
This is a diagonal approximation to the convective limit diffusion matrix (\ref{eq:convective_diffusion_scaling}).
This result is unsurprising given the use of a discrete asymptotic analysis in the derivation of AUSM$^+$-up, and almost 15 years of evidence of AUSM$^+$-up producing satisfactory results for convective low Mach number problems.
In the original paper, Liou recognised that the asymptotic analysis relies on the assumption of a uniform background pressure, and recommended that for situations where this assumption does not hold - for example shock tube problems - the low Mach number scaling factor $f_a$ should be fixed equal to one.
In this case, the diagonal coefficients $\nu_p$ and $\mu_u$ decrease and increase by an order of $M$ respectively, and the approximation $\alpha\approx-\frac{3}{4}$ is no longer valid.
The pressure splittings are now:
\begin{equation}
    \mathcal{P}^{\pm}_{(5)}(M) = \frac{1}{16} ( 8 \pm 15M \mp 10M^3 \pm 3M^5 )
\end{equation}
The resulting diffusion coefficients are:
\begin{equation}
    \nu_u \approx 0,
    \quad
    \nu_p = \frac{1}{4\rho a} \sim \mathcal{O}(M^1)
\end{equation}
\begin{equation}
    \mu_p \approx 0,
    \quad
    \mu_p \approx -\frac{21\rho a}{16} \sim \mathcal{O}(M^{-1})
\end{equation}
and the diffusion matrix scales now as:
\begin{equation}
    \underline{\underline{A}} \sim \mathcal{O}
    \begin{matrix}
    \begin{pmatrix}
        M^{-1} & 0      \\
        0      & M^{-1} \\
    \end{pmatrix}
    \end{matrix}
\end{equation}
Which is a diagonal approximation of the acoustic limit diffusion matrix (\ref{eq:acoustic_diffusion_scaling}), showing that with $f_a=1$, AUSM$^+-up$ is not only suitable for low Mach number shock tube problems, but also acoustic problems where the background pressure is constant.
