# Supplementary material for: Artificial diffusion for convective and acoustic low Mach number flows II: Application to Liou-Steffen, Zha-Bilgen and Toro-Vasquez convection-pressure flux splittings
Source: arXiv:2303.10740 source file (2023-03-19)
Supplement: Supplementary file 3 [file interface_massflux.tex]

We consider AUSM fluxes which use an interface mass flow which cannot be defined as in equation (\ref{eq:interface_mass_flow}).
Equations (\ref{eq:ausm_form2}), (\ref{eq:interface_up}) and (\ref{eq:ausm_form3}) remain the same, except for $u_{1/2}$ being replaced with $\dot{m}_{1/2}$ and $\varphi=(1, u, v, h)$.
The diffusion on the interface pressure remains unchanged from equation (\ref{eq:interface_up_diffusion}), however we add a density diffusion term to the definition of the interface mass flow, in addition to the velocity and pressure diffusion terms:
\begin{equation}
    \dot{m}_d = \varrho_p \llbracket p \rrbracket + \varrho_u \llbracket u \rrbracket + \varrho_{\rho} \llbracket \rho \rrbracket
\end{equation}
The diffusive flux Jacobian in entropy variables, equivalent to equation (\ref{eq:ausm_diffusion_symmetric}) is:
\begin{equation} \label{eq:slau_jacobian}
    \Bigg[
    \frac{\dot{m}}{\rho}
    \begin{matrix}
        \begin{pmatrix}
            \Gamma & 0 & 0 & 1 \\
            0        & 1 & 0 & 0 \\
            0        & 0 & 1 & 0 \\
            \Gamma & 0 & 0 & 1
        \end{pmatrix}
    \end{matrix}
    +
    \begin{matrix}
        \begin{pmatrix}
            a^2\varrho_p + \varrho_{\rho} & a^2\varrho_u & 0 & -\varrho_{\rho} \\
            0                             & 0            & 0 & 0 \\
            0                             & 0            & 0 & 0 \\
            0                             & 0            & 0 & 0
        \end{pmatrix}
    \end{matrix}
    +
    \begin{matrix}
        \begin{pmatrix}
            -\Gamma u \\
            1/\rho \\
            0 \\
            -\Gamma u \\
        \end{pmatrix}
    \end{matrix}
    \begin{matrix}
        \begin{pmatrix}
            \mu_p & \mu_u & 0 & 0
        \end{pmatrix} \\
        \mbox{} \\
        \mbox{} \\
        \mbox{}
    \end{matrix}
    \Bigg]
    \begin{matrix}
        \begin{pmatrix}
            \llbracket p \rrbracket \\
            \llbracket u \rrbracket \\
            \llbracket v \rrbracket \\
            \llbracket s \rrbracket
        \end{pmatrix}
    \end{matrix}
\end{equation}
The equations for $u$, $v$ and $s$ remain unchanged compared to equation (\ref{eq:ausm_diffusion_symmetric}), as does the contribution of the interface pressure diffusion to the $p$ equation.
The (1,1) and (1,4) elements of the first two matrix terms are modified compared to equation (\ref{eq:ausm_diffusion_symmetric}).
These additional terms amount to:
\begin{equation} \label{eq:massflow_extra_term}
    \frac{\dot{m}}{\rho} - \varrho_{\rho}
\end{equation}
being subtracted from the (1,1) element, and added to the (1,4) element of the complete Jacobian.
If the two terms in equation (\ref{eq:massflow_extra_term}) are approximately equal at low Mach number, then the additional terms cancel, and the interface mass flow form is equivalent to the interface velocity form.
In the SLAU flux:
\begin{equation} \label{eq:slau_density_diffusion}
    \varrho_{\rho} \approx \frac{\{\dot{m}\}}{\{\rho\}}
\end{equation}
so the additional terms (\ref{eq:massflow_extra_term}) are approximately equal, and the Jacobian (\ref{eq:slau_jacobian}) can be considered equivalent to the interface velocity form (\ref{eq:ausm_diffusion_symmetric}).
