# Supplementary material for: Artificial diffusion for convective and acoustic low Mach number flows II: Application to Liou-Steffen, Zha-Bilgen and Toro-Vasquez convection-pressure flux splittings
Source: arXiv:2303.10740 source file (2023-03-19)
Supplement: Supplementary file 4 [file non-dimensional_diffusion.tex]

The full equations are:\\

Roe-type diffusion:
\begin{subequations}
    \begin{align}
        \mathcal{R}_p & =
            \phantom{\rho}\mu_u|u|\partial_{xx}p
                + \gamma p\bigg(\frac{M^{\-2}}{\rho|v|}\mu_{11}\partial_{xx}p + \mu_{12}\partial_{xx}u\bigg)
                \phantom{+\big(M^{\-2}\mu_{21}\partial_{xx}p + \rho|v|\mu_{22}\partial_{xx}u\big)} \\
        \mathcal{R}_u & =
            \rho\mu_u|u|\partial_{xx}u
                \phantom{+ \gamma p\bigg(\frac{M^{\-2}}{\rho|v|}\mu_{11}\partial_{xx}p + \mu_{12}\partial_{xx}u\bigg)}
                +\big(M^{\-2}\mu_{21}\partial_{xx}p + \rho|v|\mu_{22}\partial_{xx}u\big) \\
        \mathcal{R}_v & = \phantom{\rho}\mu_u|u|\partial_{xx}v \\
        \mathcal{R}_s & = \phantom{\rho}\mu_u|u|\partial_{xx}s
    \end{align}
\end{subequations}

Liou-Steffen diffusion:
\begin{subequations}
    \begin{align}
        \mathcal{R}_p & =
            \phantom{\rho}\mu_u|u|\partial_{xx}p
                + \gamma p\bigg(\frac{M^{\-2}}{\rho|v|}\mu_{11}\partial_{xx}p + \mu_{12}\partial_{xx}u\bigg)
                - M^2u(\gamma-1)\big(M^{\-2}\mu_{21}\partial_{xx}p + \rho|v|\mu_{22}\partial_{xx}u\big) \\
        \mathcal{R}_u & =
            \rho\mu_u|u|\partial_{xx}u
                \phantom{+ \gamma p\bigg(\frac{M^{\-2}}{\rho|v|}\mu_{11}\partial_{xx}p + \mu_{12}\partial_{xx}u\bigg)}
                \phantom{M^2(\gamma-1)u}+ \big(M^{\-2}\mu_{21}\partial_{xx}p + \rho|v|\mu_{22}\partial_{xx}u\big) \\
        \mathcal{R}_v & =
            \phantom{\rho}\mu_u|u|\partial_{xx}v \\
        \mathcal{R}_s & =
            \rho R\gamma\mu_u|u|\partial_{xx}T
                \phantom{\gamma p\bigg(\frac{M^{\-2}}{\rho|v|}\mu_{11}\partial_{xx}p + \mu_{12}\partial_{xx}u\bigg)}
                - M^2u(\gamma-1)\big(M^{\-2}\mu_{21}\partial_{xx}p + \rho|v|\mu_{22}\partial_{xx}u\big) \\
    \end{align}
\end{subequations}

Zha-Bilgen diffusion:
\begin{subequations}
    \begin{align}
        \mathcal{R}_p & =
            \phantom{\rho}\mu_u|u|\partial_{xx}p
                \phantom{(-1)} + \gamma p\bigg(\frac{M^{\-2}}{\rho|v|}\mu_{11}\partial_{xx}p + \mu_{12}\partial_{xx}u\bigg)
                \phantom{+ \big(M^{\-2}\mu_{21}\partial_{xx}p + \rho|v|\mu_{22}\partial_{xx}u\big)} \\
        \mathcal{R}_u & =
            \rho\mu_u|u|\partial_{xx}u
                \phantom{+ (\gamma-1)p\big(\frac{M^{\-2}}{\rho|v|}\mu_{11}\partial_{xx}p + \mu_{12}\partial_{xx}u\big)}
                + \big(M^{\-2}\mu_{21}\partial_{xx}p + \rho|v|\mu_{22}\partial_{xx}u\big) \\
        \mathcal{R}_v & =
            \phantom{\rho}\mu_u|u|\partial_{xx}v \\
        \mathcal{R}_s & =
            \phantom{\rho}\mu_u|u|\partial_{xx}s
                - (\gamma-1)p\bigg(\frac{M^{\-2}}{\rho|v|}\mu_{11}\partial_{xx}p + \mu_{12}\partial_{xx}u\bigg)
    \end{align}
\end{subequations}

Toro-Vasquez diffusion:
\begin{subequations}
    \begin{align}
        \mathcal{R}_p & =
            \phantom{-\rho}\mu_u|u|\partial_{xx}p
                \phantom{- \gamma p\bigg(\frac{M^{\-2}}{\rho|v|}\mu_{11}\partial_{xx}p + \mu_{12}\partial_{xx}u\bigg)}
                + M^2u(\gamma-1)\big(M^{\-2}\mu_{21}\partial_{xx}p + \rho|v|\mu_{22}\partial_{xx}u\big) \\
        \mathcal{R}_u & =
            \phantom{-}\rho\mu_u|u|\partial_{xx}u
                \phantom{- \gamma p\bigg(\frac{M^{\-2}}{\rho|v|}\mu_{11}\partial_{xx}p + \mu_{12}\partial_{xx}u\bigg)}
                \phantom{M^2(\gamma-1)u}+ \big(M^{\-2}\mu_{21}\partial_{xx}p + \rho|v|\mu_{22}\partial_{xx}u\big) \\
        \mathcal{R}_v & = \phantom{-\rho}\mu_u|u|\partial_{xx}v \\
        \mathcal{R}_s & = -a^2\mu_u|u|\partial_{xx}\rho
                - \gamma p\bigg(\frac{M^{\-2}}{\rho|v|}\mu_{11}\partial_{xx}p + \mu_{12}\partial_{xx}u\bigg)
                + M^2u(\gamma-1)\big(M^{\-2}\mu_{21}\partial_{xx}p + \rho|v|\mu_{22}\partial_{xx}u\big) \\
    \end{align}
\end{subequations}
