# Supplementary material for: Artificial diffusion for convective and acoustic low Mach number flows II: Application to Liou-Steffen, Zha-Bilgen and Toro-Vasquez convection-pressure flux splittings
Source: arXiv:2303.10740 source file (2023-03-19)
Supplement: Supplementary file 5 [file ausm_eigenvalues.tex]

Spectral radius of upwind term:
\begin{equation}
    u : 3,
    \quad
    \gamma u : 1
\end{equation}
Spectral radius of interface velocity diffusion term:
\begin{equation}
    0 : 3,
    \quad
    \rho a^2 \nu_p : 1
\end{equation}
Spectral radius of interface pressure diffusion term:
\begin{equation}
    0 : 3,
    \quad
    \frac{\mu_u - \rho u \mu_p (\gamma-1)}{\rho} : 1
\end{equation}
Spectral radius of the combined upwinding and interface velocity diffusion:
\begin{equation}
    u : 3,
    \quad
    \gamma u + \rho a^2 \nu_p : 1
\end{equation}
Spectral radius of the combined interface velocity and pressure diffusion:
\begin{equation}
\begin{split}
    0 : 2 \\
    \frac{\mu_u - \rho u \mu_p (\gamma-1) + \rho^2 a^2 \nu_p}{2\rho} \\
    \pm \frac{\sqrt{
    \rho^4 a^4 \nu_p^2
    -2 \rho^3 a^2 u \nu_p ( \gamma - 1) \mu_p
    +2 \rho^2 a^2 ( 2 \nu_u \mu_p - \nu_p \mu_u )
    + ( \rho u \mu_p ( \gamma - 1 ) - \mu_u )^2
    }}{2\rho}
\end{split}
\end{equation}
Spectral radius of the full diffusive flux jacobian:
\begin{equation}
\begin{split}
    u : 2 \\
    \frac{\mu_u - \rho u \mu_p (\gamma-1) + \rho^2 a^2 \nu_p + \rho u (\gamma+1)}{2\rho} \\
    \pm \frac{\sqrt{
    \rho^4 a^4 \nu_p^2
    -2\rho^3 a^2 u \nu_p ( \gamma - 1 )( \mu_p - 1 )
    + 2\rho^2 a^2 ( 2 \nu_u \mu_p - \nu_p \mu_u )
    + ( \rho u \mu_p ( \gamma - 1 ) - \mu_u )^2
    + 4 \rho u \mu_u ( \gamma - 1 )
%   + \rho^2 u^2 ( \gamma - 1 )^2 ( \mu_p - 1 )^2
%   - 2\rho u \mu_u ( \gamma - 1 )( \mu_p + 1 )
%   + \mu_u^2
    }}{2\rho}
\end{split}
\end{equation}
