# Supplementary material for: Artificial diffusion for convective and acoustic low Mach number flows II: Application to Liou-Steffen, Zha-Bilgen and Toro-Vasquez convection-pressure flux splittings
Source: arXiv:2303.10740 source file (2023-03-19)
Supplement: Supplementary file 6 [file non-diagonal_limit_equations.tex]

\subsection{Roe scheme}

Limit equations at convective limit with convective diffusion for Roe.
\begin{subequations}
    \begin{align}
        \partial_t\ord{p}{0} + \gamma\ord{p}{0}\partial_x\ord{u}{0} & = \gamma\ord{p}{0}\Big( \frac{\mu_{11}}{\ord{\rho}{0}|v|}\partial_{xx}\ord{p}{2} + \mu_{12}\partial_{xx}\ord{u}{0} \Big) \\
        \ord{\rho}{0}\partial_t\ord{u}{0} + \partial_x\ord{p}{2} + \ord{\rho u}{0}\partial_x\ord{u}{0} & = \ord{\rho}{0}\mu_u|u|\partial_{xx}\ord{u}{0} + \mu_{21}\partial_{xx}\ord{p}{2} + \ord{\rho}{0}|v|\mu_{22}\partial_{xx}\ord{u}{0} \\
        \partial_t\ord{v}{0}                           +      \ord{u}{0}\partial_x\ord{v}{0} & = \mu_u|u|\partial_{xx}\ord{v}{0} \\
        \partial_t\ord{s}{0}                           +      \ord{u}{0}\partial_x\ord{s}{0} & = \mu_u|u|\partial_{xx}\ord{s}{0}
    \end{align}
\end{subequations}

Limit equations at acoustic limit with convective diffusion for Roe.
\begin{subequations}
    \begin{align}
        0 & = \gamma\ord{p}{0}\frac{\mu_{11}}{\ord{\rho}{0}|v|}\partial_{xx}\ord{p}{1} \\
        \ord{\rho}{0}\partial_{\tau}\ord{u}{0} + \partial_x\ord{p}{1} & = \mu_{21}\partial_{xx}\ord{p}{1} + \ord{\rho}{0}|v|\mu_{22}\partial_{xx}\ord{u}{0} \\
        \partial_{\tau}\ord{v}{0} & = 0 \\
        \partial_{\tau}\ord{s}{0} & = 0
    \end{align}
\end{subequations}

Limit equations at convective limit with mixed diffusion for Roe.
\begin{subequations}
    \begin{align}
        \partial_t\ord{p}{0} + \gamma\ord{p}{0}\partial_x\ord{u}{0} & =  \gamma\ord{p}{0}\mu_{12}\partial_{xx}\ord{u}{0} \\
        \ord{\rho}{0}\partial_t\ord{u}{0} + \partial_x\ord{p}{2} + \ord{\rho u}{0}\partial_x\ord{u}{0} & = \ord{\rho}{0}\mu_u|u|\partial_{xx}\ord{u}{0} + \mu_{21}\partial_{xx}\ord{p}{2} + \ord{\rho}{0}|v|\mu_{22}\partial_{xx}\ord{u}{0} \\
        \partial_t\ord{v}{0}                           +      \ord{u}{0}\partial_x\ord{v}{0} & = \mu_u|u|\partial_{xx}\ord{v}{0} \\
        \partial_t\ord{s}{0}                           +      \ord{u}{0}\partial_x\ord{s}{0} & = \mu_u|u|\partial_{xx}\ord{s}{0}
    \end{align}
\end{subequations}

Limit equations at acoustic limit with mixed diffusion for Roe.
\begin{subequations}
    \begin{align}
        \partial_{\tau}\ord{p}{0} + \gamma\ord{p}{0}\partial_x\ord{u}{0} & = \gamma\ord{p}{0}\Big(\frac{\mu_{11}}{\ord{\rho}{0}|v|}\partial_{xx}\ord{p}{1} + \mu_{12}\partial_{xx}\ord{u}{0}\Big) \\
        \ord{\rho}{0}\partial_{\tau}\ord{u}{0} + \partial_x\ord{p}{1} & = \mu_{21}\partial_{xx}\ord{p}{1} \\
        \partial_{\tau}\ord{v}{0} & = 0 \\
        \partial_{\tau}\ord{s}{0} & = 0
    \end{align}
\end{subequations}

\subsection{Liou-Steffen splitting}

Limit equations at convective limit with convective diffusion for Liou-Steffen.
\begin{subequations}
    \begin{align}
        \partial_t\ord{p}{0} + \gamma\ord{p}{0}\partial_x\ord{u}{0} & = \gamma\ord{p}{0}\Big( \frac{\mu_{11}}{\ord{\rho}{0}|v|}\partial_{xx}\ord{p}{2} + \mu_{12}\partial_{xx}\ord{u}{0} \Big) \\
        \ord{\rho}{0}\partial_t\ord{u}{0} + \partial_x\ord{p}{2} + \ord{\rho u}{0}\partial_x\ord{u}{0} & = \ord{\rho}{0}\mu_u|u|\partial_{xx}\ord{u}{0} + \mu_{21}\partial_{xx}\ord{p}{2} + \ord{\rho}{0}|v|\mu_{22}\partial_{xx}\ord{u}{0} \\
        \partial_t\ord{v}{0}                           +      \ord{u}{0}\partial_x\ord{v}{0} & = \mu_u|u|\partial_{xx}\ord{v}{0} \\
        \partial_t\ord{s}{0}                           +      \ord{u}{0}\partial_x\ord{s}{0} & = \ord{\rho}{0}\gamma R\mu_u|u|\partial_{xx}\ord{T}{0}
    \end{align}
\end{subequations}

Limit equations at acoustic limit with convective diffusion for Liou-Steffen.
\begin{subequations}
    \begin{align}
        0 & = \gamma\ord{p}{0}\frac{\mu_{11}}{\ord{\rho}{0}|v|}\partial_{xx}\ord{p}{1} \\
        \ord{\rho}{0}\partial_{\tau}\ord{u}{0} + \partial_x\ord{p}{1} & = \mu_{21}\partial_{xx}\ord{p}{1} + \ord{\rho}{0}|v|\mu_{22}\partial_{xx}\ord{u}{0} \\
        \partial_{\tau}\ord{v}{0} & = 0 \\
        \partial_{\tau}\ord{s}{0} & = 0
    \end{align}
\end{subequations}

Limit equations at convective limit with mixed diffusion for Liou-Steffen.
\begin{subequations}
    \begin{align}
        \partial_t\ord{p}{0} + \gamma\ord{p}{0}\partial_x\ord{u}{0} & =  \gamma\ord{p}{0}\mu_{12}\partial_{xx}\ord{u}{0} \\
        \ord{\rho}{0}\partial_t\ord{u}{0} + \partial_x\ord{p}{2} + \ord{\rho u}{0}\partial_x\ord{u}{0} & = \ord{\rho}{0}\mu_u|u|\partial_{xx}\ord{u}{0} + \mu_{21}\partial_{xx}\ord{p}{2} + \ord{\rho}{0}|v|\mu_{22}\partial_{xx}\ord{u}{0} \\
        \partial_t\ord{v}{0}                           +      \ord{u}{0}\partial_x\ord{v}{0} & = \mu_u|u|\partial_{xx}\ord{v}{0} \\
        \partial_t\ord{s}{0}                           +      \ord{u}{0}\partial_x\ord{s}{0} & = \ord{\rho}{0}\gamma R\mu_u|u|\partial_{xx}\ord{T}{0}
    \end{align}
\end{subequations}

Limit equations at acoustic limit with mixed diffusion for Liou-Steffen.
\begin{subequations}
    \begin{align}
        \partial_{\tau}\ord{p}{0} + \gamma\ord{p}{0}\partial_x\ord{u}{0} & = \gamma\ord{p}{0}\Big(\frac{\mu_{11}}{\ord{\rho}{0}|v|}\partial_{xx}\ord{p}{1} + \mu_{12}\partial_{xx}\ord{u}{0}\Big) \\
        \ord{\rho}{0}\partial_{\tau}\ord{u}{0} + \partial_x\ord{p}{1} & = \mu_{21}\partial_{xx}\ord{p}{1} \\
        \partial_{\tau}\ord{v}{0} & = 0 \\
        \partial_{\tau}\ord{s}{0} & = 0
    \end{align}
\end{subequations}

\subsection{Zha-Bilgen splitting}

Limit equations at convective limit with convective diffusion for Zha-Bilgen.
\begin{subequations}
    \begin{align}
        \partial_t\ord{p}{0} + \gamma\ord{p}{0}\partial_x\ord{u}{0} & = \ord{p}{0}\Big( \frac{\mu_{11}}{\ord{\rho}{0}|v|}\partial_{xx}\ord{p}{2} + \mu_{12}\partial_{xx}\ord{u}{0} \Big) \\
        \ord{\rho}{0}\partial_t\ord{u}{0} + \partial_x\ord{p}{2} + \ord{\rho u}{0}\partial_x\ord{u}{0} & = \ord{\rho}{0}\mu_u|u|\partial_{xx}\ord{u}{0} + \mu_{21}\partial_{xx}\ord{p}{2} + \ord{\rho}{0}|v|\mu_{22}\partial_{xx}\ord{u}{0} \\
        \partial_t\ord{v}{0}                           +      \ord{u}{0}\partial_x\ord{v}{0} & = \mu_u|u|\partial_{xx}\ord{v}{0} \\
        \partial_t\ord{s}{0}                           +      \ord{u}{0}\partial_x\ord{s}{0} & = \mu_u|u|\partial_{xx}\ord{s}{0} - \ord{p}{0}(\gamma-1)\Big(\frac{\mu_{11}}{\ord{\rho}{0}|v|}\partial_{xx}\ord{p}{2} + \mu_{12}\partial_{xx}\ord{u}{0}\Big) \\
    \end{align}
\end{subequations}

Limit equations at acoustic limit with convective diffusion for Zha-Bilgen.
\begin{subequations}
    \begin{align}
        0 & = \ord{p}{0}\frac{\mu_{11}}{\ord{\rho}{0}|v|}\partial_{xx}\ord{p}{1} \\
        \ord{\rho}{0}\partial_{\tau}\ord{u}{0} + \partial_x\ord{p}{1} & = \mu_{21}\partial_{xx}\ord{p}{1} + \ord{\rho}{0}|v|\mu_{22}\partial_{xx}\ord{u}{0} \\
        \partial_{\tau}\ord{v}{0} & = 0 \\
        \partial_{\tau}\ord{s}{0} & = -\ord{p}{0}(\gamma-1)\frac{\mu_{11}}{\ord{\rho}{0}|v|}\partial_{xx}\ord{p}{1}
    \end{align}
\end{subequations}

Limit equations at convective limit with mixed diffusion for Zha-Bilgen.
\begin{subequations}
    \begin{align}
        \partial_t\ord{p}{0} + \gamma\ord{p}{0}\partial_x\ord{u}{0} & =  \ord{p}{0}\mu_{12}\partial_{xx}\ord{u}{0} \\
        \ord{\rho}{0}\partial_t\ord{u}{0} + \partial_x\ord{p}{2} + \ord{\rho u}{0}\partial_x\ord{u}{0} & = \ord{\rho}{0}\mu_u|u|\partial_{xx}\ord{u}{0} + \mu_{21}\partial_{xx}\ord{p}{2} + \ord{\rho}{0}|v|\mu_{22}\partial_{xx}\ord{u}{0} \\
        \partial_t\ord{v}{0}                           +      \ord{u}{0}\partial_x\ord{v}{0} & = \mu_u|u|\partial_{xx}\ord{v}{0} \\
        \partial_t\ord{s}{0}                           +      \ord{u}{0}\partial_x\ord{s}{0} & = \mu_u|u|\partial_{xx}\ord{s}{0} - \ord{p}{0}(\gamma-1)\mu_{12}\partial_{xx}\ord{u}{0} \\
    \end{align}
\end{subequations}

Limit equations at acoustic limit with mixed diffusion for Zha-Bilgen.
\begin{subequations}
    \begin{align}
        \partial_{\tau}\ord{p}{0} + \gamma\ord{p}{0}\partial_x\ord{u}{0} & = \ord{p}{0}\Big(\frac{\mu_{11}}{\ord{\rho}{0}|v|}\partial_{xx}\ord{p}{1} + \mu_{12}\partial_{xx}\ord{u}{0}\Big) \\
        \ord{\rho}{0}\partial_{\tau}\ord{u}{0} + \partial_x\ord{p}{1} & = \mu_{21}\partial_{xx}\ord{p}{1} \\
        \partial_{\tau}\ord{v}{0} & = 0 \\
        \partial_{\tau}\ord{s}{0} & = 0
    \end{align}
\end{subequations}

\subsection{Toro-Vasquez splitting}

Limit equations at convective limit with convective diffusion for Toro-Vasquez.
\begin{subequations}
    \begin{align}
        \partial_t\ord{p}{0} + \gamma\ord{p}{0}\partial_x\ord{u}{0} & = 0 \\
        \ord{\rho}{0}\partial_t\ord{u}{0} + \partial_x\ord{p}{2} + \ord{\rho u}{0}\partial_x\ord{u}{0} & = \ord{\rho}{0}\mu_u|u|\partial_{xx}\ord{u}{0} + \mu_{21}\partial_{xx}\ord{p}{2} + \ord{\rho}{0}|v|\mu_{22}\partial_{xx}\ord{u}{0} \\
        \partial_t\ord{v}{0}                           +      \ord{u}{0}\partial_x\ord{v}{0} & = \mu_u|u|\partial_{xx}\ord{v}{0} \\
        \partial_t\ord{s}{0}                           +      \ord{u}{0}\partial_x\ord{s}{0} & = -a^2\mu_u|u|\partial_{xx}\ord{\rho}{0} - \gamma\ord{p}{0}\Big( \frac{\mu_{11}}{\ord{\rho}{0}|v|}\partial_{xx}\ord{p}{2} + \mu_{12}\partial_{xx}\ord{u}{0} \Big)
    \end{align}
\end{subequations}

Limit equations at acoustic limit with convective diffusion for Toro-Vasquez.
\begin{subequations}
    \begin{align}
        \partial_{\tau}\ord{p}{0} + \gamma\ord{p}{0}\partial_x\ord{u}{0} & = 0 \\
        \ord{\rho}{0}\partial_{\tau}\ord{u}{0} + \partial_x\ord{p}{1} & = \mu_{21}\partial_{xx}\ord{p}{1} + \ord{\rho}{0}|v|\mu_{22}\partial_{xx}\ord{u}{0} \\
        \partial_{\tau}\ord{v}{0} & = 0 \\
        \partial_{\tau}\ord{s}{0} & =  -\gamma\ord{p}{0}\frac{\mu_{11}}{\ord{\rho}{0}|v|}\partial_{xx}\ord{p}{1}
    \end{align}
\end{subequations}

Limit equations at convective limit with mixed diffusion for Toro-Vasquez.
\begin{subequations}
    \begin{align}
        \partial_t\ord{p}{0} + \gamma\ord{p}{0}\partial_x\ord{u}{0} & = 0 \\
        \ord{\rho}{0}\partial_t\ord{u}{0} + \partial_x\ord{p}{2} + \ord{\rho u}{0}\partial_x\ord{u}{0} & = \ord{\rho}{0}\mu_u|u|\partial_{xx}\ord{u}{0} + \mu_{21}\partial_{xx}\ord{p}{2} + \ord{\rho}{0}|v|\mu_{22}\partial_{xx}\ord{u}{0} \\
        \partial_t\ord{v}{0}                           +      \ord{u}{0}\partial_x\ord{v}{0} & = \mu_u|u|\partial_{xx}\ord{v}{0} \\
        \partial_t\ord{s}{0}                           +      \ord{u}{0}\partial_x\ord{s}{0} & = -a^2\mu_u|u|\partial_{xx}\ord{\rho}{0} - \gamma\ord{p}{0}\mu_{12}\partial_{xx}\ord{u}{0}
    \end{align}
\end{subequations}

Limit equations at acoustic limit with mixed diffusion for Toro-Vasquez.
\begin{subequations}
    \begin{align}
        \partial_{\tau}\ord{p}{0} + \gamma\ord{p}{0}\partial_x\ord{u}{0} & = 0 \\
        \ord{\rho}{0}\partial_{\tau}\ord{u}{0} + \partial_x\ord{p}{1} & = \mu_{21}\partial_{xx}\ord{p}{1} \\
        \partial_{\tau}\ord{v}{0} & = 0 \\
        \partial_{\tau}\ord{s}{0} & = 0
    \end{align}
\end{subequations}
